# Supplementary material for: Personalized Recommendations in EdTech: Evidence from a Randomized Controlled Trial
Source: arXiv:2208.13940 source file (2022-12-04)
Supplement: Supplementary file 1 [file outliers_appendix.tex]

\section{Instrumentation errors}
Variables measuring utilization of the app are derived from raw log-files of Stones2Milestones. This data is the most accurate, available representation of users' activity on the app. Nevertheless, there are occasional instrumentation errors. Here, we focus on errors in classification of user-story interaction outcome. Some users will have their interactions labeled as having completed a story, even though, they would have merely clicked on it to view. Such users will end up having a high and spurious utilization of the app. 

Even though we do not have a reason to believe that such events are more widespread in either of the experimental groups, they introduce noise to the data, which in this specific case translate into higher standard errors of estimated statistics.
